# Supplementary material for: GIN: Graph-based Interaction-aware Constraint Policy Optimization for Autonomous Driving
Source: arXiv:2206.01488 source file (2022-08-24)
Supplement: Supplementary file 1 [file appendix.tex]

\section*{APPENDIX}

Appendixes should appear before the acknowledgment.
